# Supplementary material for: Learn to Optimize Denoising Scores for 3D Generation: A Unified and Improved Diffusion Prior on NeRF and 3D Gaussian Splatting
Source: arXiv:2312.04820 source file (2023-12-08)
Supplement: Supplementary file 1 [file _supplementary.tex]

\input{_constants}
\review % \review OR \cameraready

\documentclass[10pt,twocolumn,letterpaper]{article}
\input{cvpr_header}
\myexternaldocument{_main}
\begin{document}

%% TITLE
\title{\paperTitle}
\author{\authorBlock}
\maketitlesupplementary

\input{12_appendix}

{\small
\bibliographystyle{ieeenat_fullname}
\bibliography{11_references}
}

\end{document}
